# Supplementary material for: Locality-aware Gaussian Compression for Fast and High-quality Rendering
Source: arXiv:2501.05757 source file (2025-03-12)
Supplement: Supplementary file 1 [file ratio.tex]

\begin{figure*}[!ht]
\begin{center}
\includegraphics[width=\linewidth]{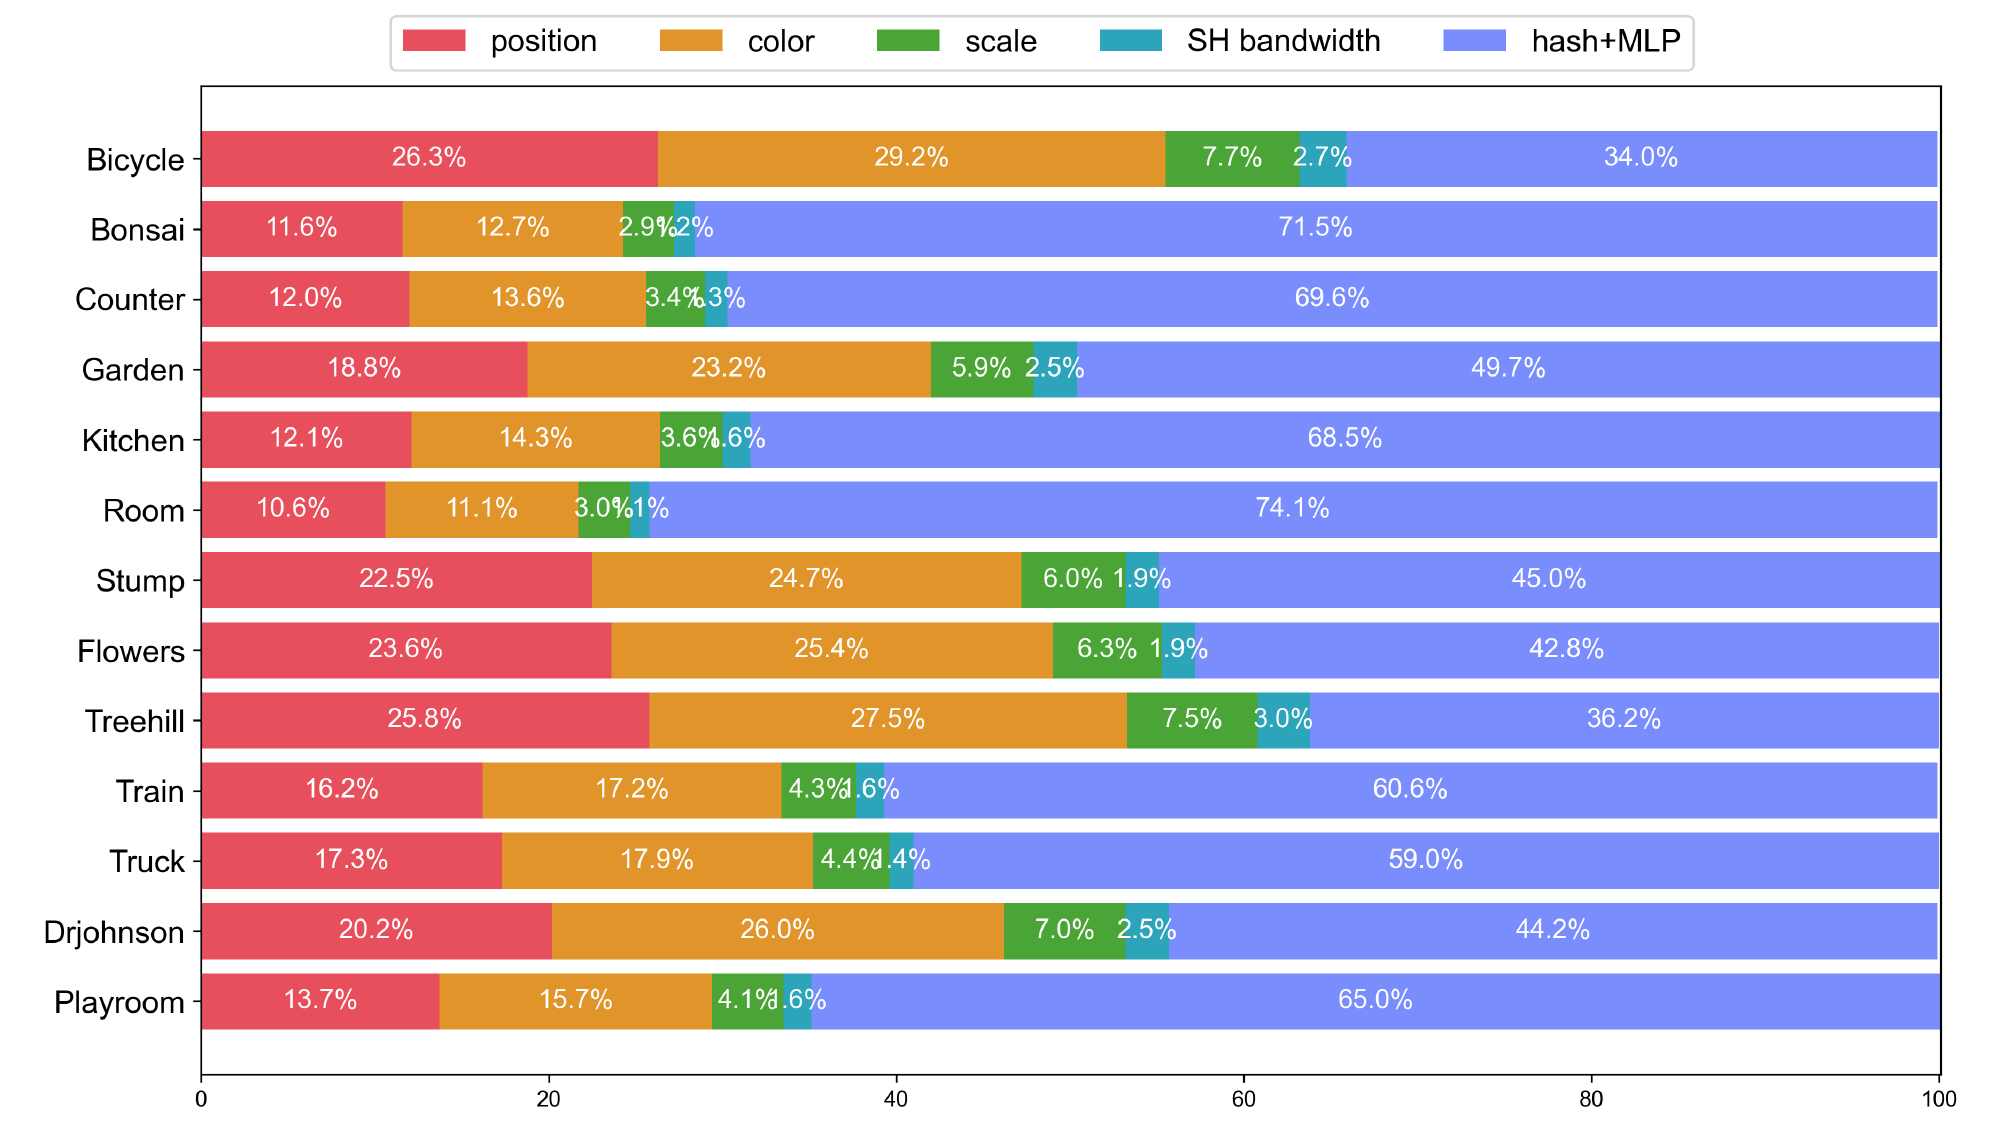}
\end{center}
\vspace{-4mm}
\caption{Analysis of the storage size for each component of our representation.}
% \vspace{-4mm}
\label{fig:ratio}
\end{figure*}
