# Supplementary material for: Locality-aware Gaussian Compression for Fast and High-quality Rendering
Source: arXiv:2501.05757 source file (2025-03-12)
Supplement: Supplementary file 2 [file experimental_setting.tex]

\subsection{Detailed Experimental Setting}

\subsection{Dataset}
We employ three real-world 3D datasets, the Mip-NeRF 360 dataset~\cite{barron2022mip}, Tanks and Temples~\cite{knapitsch2017tanks}, and Deep Blending dataset~\cite{hedman2018deep}. The authors of 3D Gaussian Splatting (3DGS)~\cite{kerbl20233d} offers pre-processed Tanks and Temples dataset and Deep Blending dataset, while employs 
All images are resized to a maximum width of 1.6K pixels while maintaining their original aspect ratio~\cite{kerbl20233d}.

\subsection{Dataset}
